# Supplementary material for: You Can Do Better! If You Elaborate the Reason When Making Prediction
Source: arXiv:2103.14919 source file (2021-05-29)
Supplement: Supplementary file 1 [file appendix.tex]

\appendix

% \section{Appendix}
\label{sec:supplemental}

\section{Details of Input-Output Formats}

\begin{table*}[!ht]
\centering
\small
\begin{tabular}{p{\textwidth}}
\toprule
\textbf{The \textit{y}$|$\textit{x} classifier inputs}:\\
for i$_{th}$ option: $[CLS] \{question\} [SEP] \{option_i\} [EOS]$ \\
\midrule
\textbf{The \textit{y}$|$(\textit{x}, \textit{evidence}) classifier inputs}:\\
for i$_{th}$ option: $[CLS] \{question\} \{option_i\} [SEP] \{evidence_i\} [EOS]$ \\
\midrule
\textbf{The \textit{y}$|$(\textit{x}, \textit{expls}) classifier inputs}:\\
for i$_{th}$ option: $[CLS] \{question\} \{option_i\} [SEP] \{golden\_explanations_i\} [EOS]$ \\
\midrule
\textbf{To calculate Accuracy$_{y_e}$ when test, the classifier inputs}:\\
for i$_{th}$ option: $[CLS] \{option_i\} [SEP] \{explanations_i\} [EOS]$ \\
\midrule
\textbf{The generator inputs is}:\\
$[CLS] \{question\}\ The\ options\ are\ \{option_1\} \{option_2\} ... reference: \{question\_context\} [SEP]$ \\
\midrule
\textbf{The generator inputs without question context}:\\
$[CLS] \{question\}\ The\ options\ are\ \{option_1\} \{option_2\} ... [SEP]$ \\
\midrule
\textbf{The generator outputs}:\\
My commonsense tells me that \{generated explanation\}.\\
\bottomrule
\end{tabular}
\caption{The input-output formatting of each variant. Here $[CLS]$, $[SEP]$ and $[EOS]$ mean symbols for segmentation, and depend on different pre-trained models.}
\vspace{-2mm}
\label{tab:t5_data_format}
\end{table*}

The inputs and outputs are different text sequences. And we provide the input-output formatting of training and decoding of each variant in Table~\ref{tab:t5_data_format}. 

\section{Examples of Generated Explanations}
We list the explanations generated for five random test examples, along with the input and golden labels from three datasets. Besides, the batch size of these dataset in training is set to \{$16$, $4$, $4$\} and the gradient accumulation step is set to $4$. 
\subsection{e-SNLI}
% In our work, we have taken a step further and built a neural network that is able to directly provide full-sentence natural language justifications. There has been little work on incorporating and outputting natural language free-form explanations, mostly due to the lack of appropriate datasets. In this direction, and very similar to our approach, is the recent work by Park et al. [23], who introduce two datasets of natural language explanations for the tasks of visual question-answering and activity recognition. Another work in this direction is that of Ling et al. [18], who introduced a dataset of textual justifications for solving math problems and formulate the task in terms of program execution. Nonetheless, their setup is specific to the task of solving math problems, and thus hard to transfer to more general natural understanding tasks. Jansen et al. [16] provided a dataset of natural language explanation graphs for elementary science questions. However, with only 1, 680 pairs of questions and explanations, their corpus is orders of magnitude smaller than e-SNLI. 
Examples in training set where the explanations include the whole text of the premise or hypothesis are droped.~\footnote{\url{https://github.com/SawanKumar28/nile/}} We also used the first two explanations as references for BLEU calculation of generated explanations. Here we list some examples from test set. The means and standard deviations of performance of our method on e-SNLI development set is $92.91$ and $0.05$. 
\begin{itemize}[]
	\item \textbf{{Id}}: 2677109430.jpg\#1r1n \\
	\textbf{{Golden label}}: neutral \\
	\textbf{{Premise}}: This church choir sings to the masses as they sing joyous songs from the book at a church. \\
	\textbf{{Hypothesis}}: The church has cracks in the ceiling. \\
	\textbf{{Generated Explanation}}: The church choir singing joyous songs from the book does not imply that the church has cracks in the ceiling.\\
    \textbf{{Golden Explanation}}: Not all churches have cracks in the ceiling. 
\end{itemize}
\begin{itemize}[]
	\item \textbf{{Id}}: 6160193920.jpg\#4r1c \\
	\textbf{{Golden label}}: contradiction \\
	\textbf{{Premise}}: A woman with a green headscarf, blue shirt and a very big grin. \\
	\textbf{{Hypothesis}}: The woman has been shot.  \\
	\textbf{{Generated Explanation}}: A woman with a green headscarf does not imply she has been shot.\\
	\textbf{{Golden Explanation}}: There can be either a woman with a very big grin or a woman who has been shot.
\end{itemize}
\begin{itemize}[]
%  29
	\item \textbf{{Id}}: 3572548523.jpg\#4r1n \\ 
	\textbf{{Golden label}}: neutral \\
	\textbf{{Premise}}: A couple walk hand in hand down a street. \\
	\textbf{{Hypothesis}}: The couple is married.  \\
	\textbf{{Generated Explanation}}: Not all couples are married.\\
	\textbf{{Golden Explanation}}: Just because the couple is hand in hand doesn't mean they are married.
\end{itemize}
\begin{itemize}[]
	\item \textbf{{Id}}: 2936881937.jpg\#2r1e \\
	\textbf{{Golden label}}: entailment \\
	\textbf{{Premise}}: A man in a black shirt is looking at a bike in a workshop. \\
	\textbf{{Hypothesis}}: A man is in a black shirt  \\
	\textbf{{Generated Explanation}}: The man in a black shirt is looking at the bike.\\
	\textbf{{Golden Explanation}}: A man in a black shirt is the same as a man who is in a black shirt.
\end{itemize}

\begin{itemize}[]
% contradiction,A dog jumping for a Frisbee in the snow.,A cat washes his face and whiskers with his front paw.
	\item \textbf{{Id}}: 3338217927.jpg\#2r1c \\
	\textbf{{Golden label}}: contradiction \\
	\textbf{{Premise}}: A dog jumping for a Frisbee in the snow. \\
	\textbf{{Hypothesis}}: A cat washes his face and whiskers with his front paw.  \\
	\textbf{{Generated Explanation}}: A dog is not a cat.\\
	\textbf{{Golden Explanation}}: Dogs and cats are not the same animal, and they are performing different activities: the dog jumps while the cat engages in cleaning himself.
\end{itemize}

\subsection{CoS-E}
% The CoS-E dataset includes many meaningless and uninformative explanations, such as "I consider it the best option because they have to be more true." These can affect the generation of the model, and more evaluation needs to be done. Nevertheless, our model is able to generate some text that is relevant to the prediction.
We list five examples in the development set of v1.0 version includes model-generated texts, the original input, and golden explanations. 
\begin{itemize}[]
% contradiction,A dog jumping for a Frisbee in the snow.,A cat washes his face and whiskers with his front paw.
% "predict_explanation": "joe and mac were playing basketball to have fun.",
    % "golden_explanation": "playing basketball is also have fun"
    % Joe and Mac were playing basketball. They did it every day in their back yard.  Why were they playing basketball?,cheers,pain,have fun,2
	\item \textbf{{Id}}: f2645d0ee8662b6553954cee7e77979e \\
	\textbf{{Golden label}}: 2 \\
	\textbf{{Question}}: Joe and Mac were playing basketball. They did it every day in their back yard.  Why were they playing basketball? \\
	\textbf{{Options}}: cheers; pain; have fun  \\
	\textbf{{Generated Explanation}}: Joe and mac were playing basketball to have fun.\\
	\textbf{{Golden Explanation}}: Playing basketball is also have fun
\end{itemize}
\begin{itemize}[]
	\item \textbf{{Id}}: 22458fdcead20e2def0df0d92d5806f6 \\
	\textbf{{Golden label}}: 0 \\
	\textbf{{Question}}: WHere do people live? \\
	\textbf{{Options}}: surface of earth; bus depot; football stadium  \\
	\textbf{{Generated Explanation}}: People live on the surface of earth\\
	\textbf{{Golden Explanation}}: Surface of earth  people live?
\end{itemize}

\begin{itemize}[]
	\item \textbf{{Id}}: 21763a65765b5405c9a54484c2e54a72 \\
	\textbf{{Golden label}}: 0 \\
	\textbf{{Question}}: Where are people likely to become impatient? \\
	\textbf{{Options}}: end of line; neighbor's house; buildings  \\
	\textbf{{Generated Explanation}}: I consider it the best option because they have to be more true\\
	\textbf{{Golden Explanation}}: But it doesn't help us understand why we become impatient, what triggers the ... it's likely he didn't know how much it would hurt to climb the hill. ... in contrast, some people are overly
\end{itemize}
% ,,0,airplane have windshield

\begin{itemize}[]
	\item \textbf{{Id}}: f7a6d0d816d14210f3af5dabe21bf804 \\
	\textbf{{Golden label}}: 0 \\
	\textbf{{Question}}: What is unlikely to get bugs on its windshield due to bugs' inability to reach it when it is moving? \\
	\textbf{{Options}}: airplane; motorboat; motor vehicle  \\
	\textbf{{Generated Explanation}}: Airplanes are unlikely to have bugs on their windshields\\
	\textbf{{Golden Explanation}}: Airplane have windshield
\end{itemize}

\begin{itemize}[]
	\item \textbf{{Id}}: 6e433471d0e2590b8c73ceef275022b1 \\
	\textbf{{Golden label}}: 1\\
	\textbf{{Question}}: James knew that he shouldn't have been buying beer for minors.  He didn't even get paid for it.  Why was this bad? \\
	\textbf{{Options}}: lose money; broken law; have no money  \\
	\textbf{{Generated Explanation}}: He didn't get paid for it.\\
	\textbf{{Golden Explanation}}: By buying beer for minors james breaks the law.
\end{itemize}
% 6e433471d0e2590b8c73ceef275022b1,J,lose money,broken law,have no money,1,
% 21763a65765b5405c9a54484c2e54a72,,,0,""

% WHere do people live?,surface of earth,bus depot,football stadium,0,surface of earth  people live?
% \section{Human Evaluation GUI}
% as supplement materials
\subsection{CME}
Most of the topics in our CME dataset are related to comprehensive knowledge of pharmacy. 
% We include problems from both real exams and mock tests; all are freely accessible online for public usage. 
In terms of causality, we further did human evaluation with all test examples. The results are summarized in Table~\ref{tab:cme}. 
\begin{table}[ht]
\small
\centering
\begin{tabular}{lccc}
\toprule
Method                   & Win  & Lose & Tie  \\
\midrule
Ours vs. Human           & 0.07 & 0.50 & 0.43 \\
% \midrule
Ours vs. Only Generation & 0.19 & 0.17 & 0.63 \\
% \midrule
Ours vs. WT5             & 0.26 & 0.17 & 0.57 \\
\midrule
Cohen's kappa coefficient & \multicolumn{3}{c}{$0.5566$}  \\
\bottomrule
\end{tabular}
\caption{Human evaluation results in terms of causality.}
    % \vspace{-mm}
\label{tab:cme}
\end{table}
Moreover, we list five random examples that are better than human-generated explanations. The English version of the generated explanation is automatically translated by Google Translate~\footnote{\url{https://translate.google.com/}}. 
\begin{itemize}[]
	\item \textbf{{Id}}: 0 \\
	\textbf{{Golden label}}: C\\
	\textbf{{Question}}: \begin{CJK}{UTF8}{gbsn}患者接受顺铂化疗时，药师应重点监测的不良反应是？\end{CJK} When a patient receives cisplatin chemotherapy, which adverse reaction should the pharmacist focus on monitoring?\\
	\textbf{{Options}}: \begin{CJK}{UTF8}{gbsn}A. 心脏毒性; B. 肝脏毒性; C. 肾脏毒性; D. 肺纤维化; E. 过敏反应\end{CJK} A. Cardiotoxicity; B. Liver toxicity; C. Kidney toxicity; D. Pulmonary fibrosis; E. Allergic reaction  \\
	\textbf{{Generated Explanation}}: \begin{CJK}{UTF8}{gbsn}顺铂是肾毒性药物,可降低肾小球滤过率,影响博来霉素的清除率。\end{CJK} Cisplatin is a nephrotoxic drug, which can reduce the glomerular filtration rate and affect the clearance rate of bleomycin.\\
	\textbf{{Golden Explanation}}: \begin{CJK}{UTF8}{gbsn}部分抗肿瘤药物具有特殊毒性反应，例如顺铂的耳、肾、神经毒性显著；蔥环类抗生素（多柔比星、表柔比星、米托蔥醌等）的心脏毒性明显；甲氨蝶呤的肺纤维化毒性较大；环磷酰胺和异环磷酰胺可引起出血性膀胱炎；紫杉醇、门冬酰胺酶容易引起过敏反应；伊立替康导致腹泻较严重。\end{CJK} Some anti-tumor drugs have special toxic reactions, for example, the ear, kidney, and neurotoxicity of the cisplatin is significant; allium ring antibiotics (doxorubicin, epirubicin, mitoxonquinone, etc.) have obvious cardiotoxicity; methotrexate Cyclophosphamide and ifosfamide can cause hemorrhagic cystitis; paclitaxel and asparaginase are prone to allergic reactions; irinotecan causes more severe diarrhea.
\end{itemize}
\begin{itemize}[]
	\item \textbf{{Id}}: 16 \\
	\textbf{{Golden label}}: D\\
	\textbf{{Question}}: \begin{CJK}{UTF8}{gbsn}通过产生抗病毒蛋白，抑制病毒的复制，但无直接杀灭病毒作用的乙肝治疗药物是？\end{CJK} What is the hepatitis B treatment drug that inhibits virus replication by producing antiviral protein, but does not have the direct effect of killing the virus?\\
	\textbf{{Options}}: \begin{CJK}{UTF8}{gbsn}A. 谷胱甘肽; B. 替比夫定; C. 替诺福韦; D. α-干扰素; E. 甘草酸制剂\end{CJK} A. Glutathione; B. Telbivudine; C. Tenofovir; D. Alpha-interferon; E. Glycyrrhizic acid preparations  \\
	\textbf{{Generated Explanation}}:\begin{CJK}{UTF8}{gbsn}α-干扰素通过产生抗病毒蛋白,抑制病毒的复制,但无直接杀灭病毒作用。\end{CJK} Alpha-interferon inhibits virus replication by producing antiviral protein, but has no direct effect on killing the virus.\\
	\textbf{{Golden Explanation}}: \begin{CJK}{UTF8}{gbsn}α-干扰素有广谱的抗病毒作用，作用机制是通过产生抗病毒蛋白，可以抑制病毒复制，对病毒并无直接的杀灭作用。核昔酸类似物主要抑制病毒聚合酶或逆转录酶，从而抑制病毒DNA的合成和增殖，常见药物有拉米夫定、阿徳福韦,恩替卡韦、替比夫定、替诺福韦\end{CJK} Alpha-interferon has a broad-spectrum antiviral effect. The mechanism of action is to inhibit virus replication by producing antiviral proteins, but has no direct killing effect on the virus. Nucleotide analogs mainly inhibit viral polymerase or reverse transcriptase, thereby inhibiting the synthesis and proliferation of viral DNA. Common drugs include lamivudine, adefovir, entecavir, telbivudine, and tenofovir
\end{itemize}
\begin{itemize}[]
	\item \textbf{{Id}}: 40 \\
	\textbf{{Golden label}}: A\\
	\textbf{{Question}}:\begin{CJK}{UTF8}{gbsn} 因胰腺功能不全引起的消化不良性腹泻适宜选用？\end{CJK} Which one is suitable for dyspeptic diarrhea caused by pancreatic insufficiency? \\
	\textbf{{Options}}: \begin{CJK}{UTF8}{gbsn} A. 胰酶片; B. 碳酸氢钠; C. 胃蛋白酶; D. 地芬诺酯; E. 鞣酸蛋白\end{CJK} A. Pancreatin Tablets; B. Sodium Bicarbonate; C. Pepsin; D. Diphenoxylate; E. Tannin  \\
	\textbf{{Generated Explanation}}:\begin{CJK}{UTF8}{gbsn} 2.对消化和吸收不良综合征,因胰腺功能不全引起的消化不良性腹泻患者,应用胰酶替代疗法。\end{CJK} 2. For patients with digestive and malabsorption syndromes and dyspeptic diarrhea caused by pancreatic insufficiency, pancreatic enzyme replacement therapy should be used.\\
	\textbf{{Golden Explanation}}: \begin{CJK}{UTF8}{gbsn}因胰腺功能不全所致消化不良性腹泻应服用胰酶：对摄食脂肪过多者可服用胰酶和碳酸氢钠；对摄食蛋白而致消化不良者宜服胃蛋白酶；对同时伴腹胀者可选用乳酶生或二甲硅油。\end{CJK} Pancreatic enzymes should be administered for dyspeptic diarrhea due to pancreatic insufficiency: pancreatic enzymes and sodium bicarbonate may be used for those with excessive fat intake, pepsin may be used for those with dyspepsia due to ingested protein, and lactase or simethicone may be used for those with simultaneous abdominal distension.
\end{itemize}
\begin{itemize}[]
	\item \textbf{{Id}}: 77 \\
	\textbf{{Golden label}}: A\\
	\textbf{{Question}}: \begin{CJK}{UTF8}{gbsn}甲氧氯普胺可引起的药源性疾病是？\end{CJK} Which is the pharmacogenetic disease that metoclopramide can cause?\\
	\textbf{{Options}}: \begin{CJK}{UTF8}{gbsn}A. 锥体外系反应; B. 癫痫发作; C. 肝功能受损; D. 血小板减少症; E. 缺血性结肠炎\end{CJK} A. Extrapyramidal response; B. Seizure; C. Impaired liver function; D. Thrombocytopenia; E. Ischemic colitis \\
	\textbf{{Generated Explanation}}: \begin{CJK}{UTF8}{gbsn}甲氧氯普胺可引起的药源性疾病是锥体外系反应。\end{CJK} The pharmacogenic disease that metoclopramide can cause is an extrapyramidal reaction.\\
	\textbf{{Golden Explanation}}: \begin{CJK}{UTF8}{gbsn}1.可引起锥体外系反应的药物：氯丙嗪及其衍生物的锥体外系反应发生率高。此外利血平、氟哌啶醇、五氟利多、甲基多巴、左旋多巴、碳酸锂、甲氧氯普胺和吡罗昔康等也可致锥体外系反应。\end{CJK} 1. Drugs that can cause extrapyramidal reactions: chlorpromazine and its derivatives have a high incidence of extrapyramidal reactions.In addition reserpine, haloperidol, pentafluorolido, methyldopa, levodopa, lithium carbonate, metoclopramide and piroxicam can also cause extrapyramidal reactions.
\end{itemize}
\begin{itemize}[]
	\item \textbf{{Id}}: 106 \\
	\textbf{{Golden label}}: C\\
	\textbf{{Question}}: \begin{CJK}{UTF8}{gbsn}长期服用，可导致药源性咳嗽的药物是？\end{CJK} Which drug can cause a pharmacogenic cough when taken chronically? \\
	\textbf{{Options}}: \begin{CJK}{UTF8}{gbsn}A. 苯丙哌林; B. 右美沙芬; C. 卡托普利; D. 羧甲司坦; E. 替米沙坦 \end{CJK} A. Phenprocoumon; B. Dextromethorphan; C. Captopril; D. Carboxymestane; E. Telmisartan \\
	\textbf{{Generated Explanation}}: \begin{CJK}{UTF8}{gbsn}卡托普利可导致药源性咳嗽。\end{CJK} Captopril can cause a pharmacogenic cough.\\
	\textbf{{Golden Explanation}}: \begin{CJK}{UTF8}{gbsn}血管紧张素转换酶抑制剂可抑制缓激肽降解，造成缓激肽过多，引起干咳。血管紧张素Ⅱ受体拮抗剂没有这个毒副作用。\end{CJK} Angiotensin converting enzyme inhibitors can inhibit bradykinin degradation, causing bradykinin excess, causing dry cough. Angiotensin II receptor antagonists do not have this toxic side effect.
\end{itemize}
